# Supplementary material for: 3D Equivariant Diffusion for Target-Aware Molecule Generation and Affinity Prediction
Source: arXiv:2303.03543 source file (2023-03-06)
Supplement: Supplementary file 1 [file suppl_properties.tex]

\begin{tabular}{c|cc|cc|cc|cc}
\toprule
\diagbox{Model}{Metric} & \multicolumn{2}{c|}{High Affinity ($\uparrow$)} & \multicolumn{2}{c|}{QED ($\uparrow$)}   & \multicolumn{2}{c|}{SA ($\uparrow$)} & \multicolumn{2}{c}{Diversity ($\uparrow$)} \\
 & Avg. & Med. & Avg. & Med. & Avg. & Med. & Avg. & Med.  \\
\midrule
GraphBP       & 14.2\% & 6.7\% & 0.43 & 0.45 & 0.49 & 0.48 & 0.79 & 0.78 \\
Pocket2Mol  & 49.8\% & 52.0\% & 0.56 & 0.57 & 0.74 & 0.75 & 0.69 & 0.71 \\
TargetDiff  & 51.3\% & 50.0\% & 0.48 & 0.48 & 0.58 & 0.58 & 0.72 & 0.71 \\
Reference   & -      & -      & 0.48 & 0.47 & 0.73 & 0.74 & -    & -    \\
\bottomrule
\end{tabular}
